# Supplementary material for: Tuning proximity-induced spin-orbit coupling in graphene/WSe$_{2}$ heterostructures
Source: arXiv:2512.02522 source file (2026-06-10)
Supplement: Supplementary file 1 [file TwistedGraphene_Rockinger_Suppl.pdf]

# Supplementary Material
# Tuning proximity-induced spin-orbit coupling in graphene/$WSe_2$ heterostructures

Tobias Rockinger,[1] Bálint Szentpéteri,[2,3] Szabolcs Csonka,[2,4] Marina Marocko,[1] Julia Amann,[1] Ziyang Gan,[5] Antony George,[5] Andrey Turchanin,[5] Kenji Watanabe,[6] Takashi Taniguchi,[7] Dieter Weiss,[1] Péter Makk,[2,3] and Jonathan Eroms[1]

[1]*Institut of Experimental and Applied Physics, University of Regensburg, 93040 Regensburg, Germany*
[2]*Department of Physics, Budapest University of Technology and Economics, Műegyetem rkp. 3., 1111 Budapest, Hungary*
[3]*MTA-BME Correlated van der Waals Structures Momentum Research Group, Műegyetem rkp. 3., 1111 Budapest, Hungary*
[4]*MTA-BME Superconducting Nanoelectronics Momentum Research Group, Műegyetem rkp. 3., 1111 Budapest, Hungary*
[5]*Institute of Physical Chemistry, Friedrich Schiller University Jena, 07743 Jena, Germany*
[6]*Research Center for Electronic and Optical Materials, National Institute for Materials Science, 1-1 Namiki, Tsukuba 305-0044, Japan*
[7]*Research Center for Materials Nanoarchitectonics, National Institute for Materials Science, 1-1 Namiki, Tsukuba 305-0044, Japan*

(Dated: December 1, 2025)

In this document, we show additional data of the samples under study. Transport characterization of samples 2 to 6 at $B = 0$ is reported in Fig. S1, and momentum relaxation times and diffusion constants for all samples are given in Fig. S2. Magnetoconductance curves showing WAL are plotted in Fig. S3 for samples 2 to 6, together with fitting curves. The corresponding fitting parameters for samples 4 to 6 can be found in Fig. S4 (while the data for samples 1 to 3 are given in the main text). Finally, in Fig. S5 we show the magnetoconductance curves for the high-pressure experiments, while the extracted parameters are again shown in the main text.

## S.1.
## FURTHER DATA - TWIST ANGLE DEPENDENCE OF THE SOC

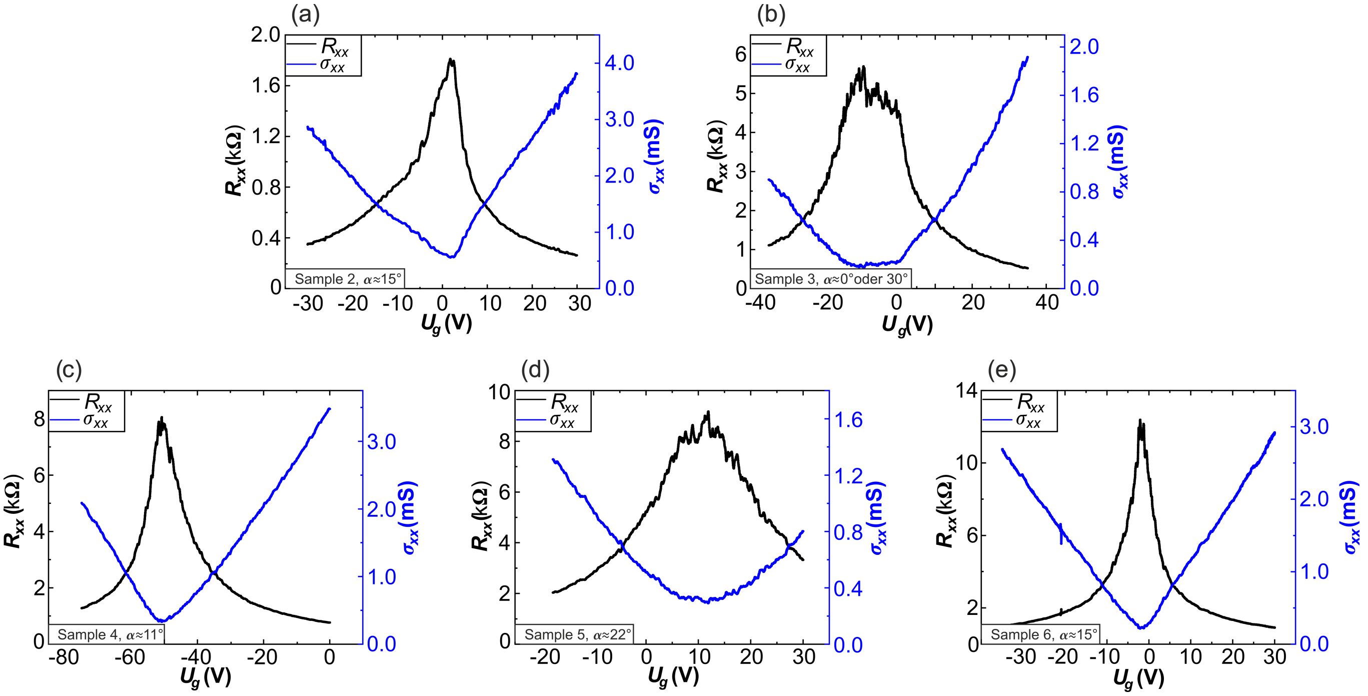


FIG. S 1. (a)-(e) four-point resistance $R_{xx}$ and conductivity $\sigma_{xx}$ near the Dirac points for samples 2-6 as a function of the gate voltage $U_g$.

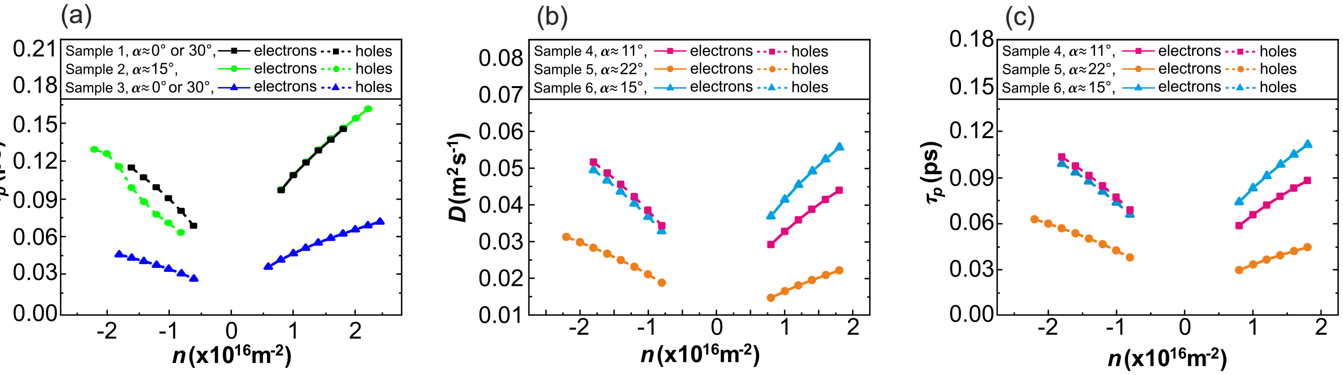


FIG. S 2. (a) Momentum relaxation time $\tau_p$ for samples 1-3 as a function of the charge carrier density $n$. (b)-(c) Momentum relaxation time $\tau_p$ and diffusion coefficient $D$ for samples 4-6 as a function of the charge carrier density $n$.

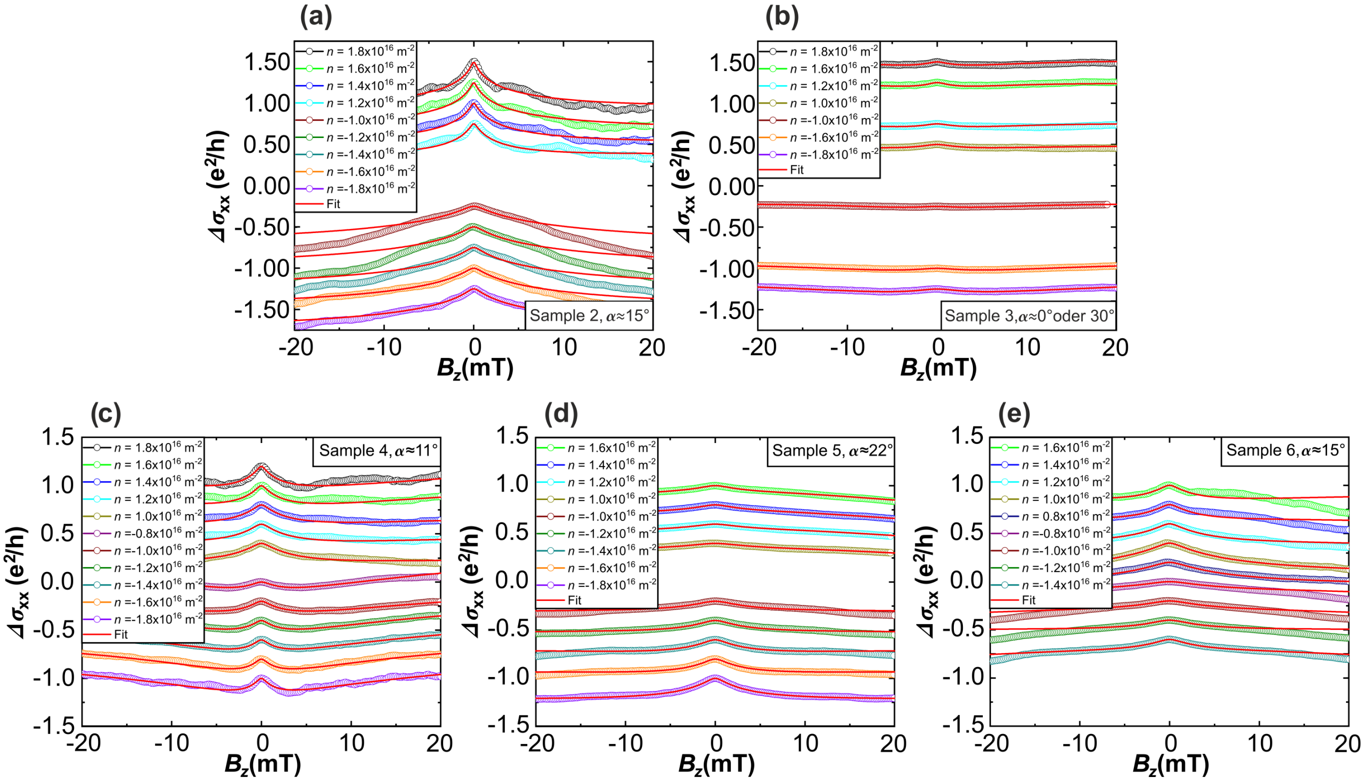


FIG. S 3. (a)-(e) Measurements of the quantum mechanical correction of the conductivity $\Delta\sigma_{xx}$ as a function of an external magnetic field $B_z$ for five samples. Some curves show how the Berry-WAL changes into the SOC-WAL. Other curves show a transition from weak localization to SOC-WAL. The red curves represent possible fit curves. Some curves are also missing for certain charge carrier densities $n$, as in these cases no suitable fit could be created or no transport parameters could be determined.

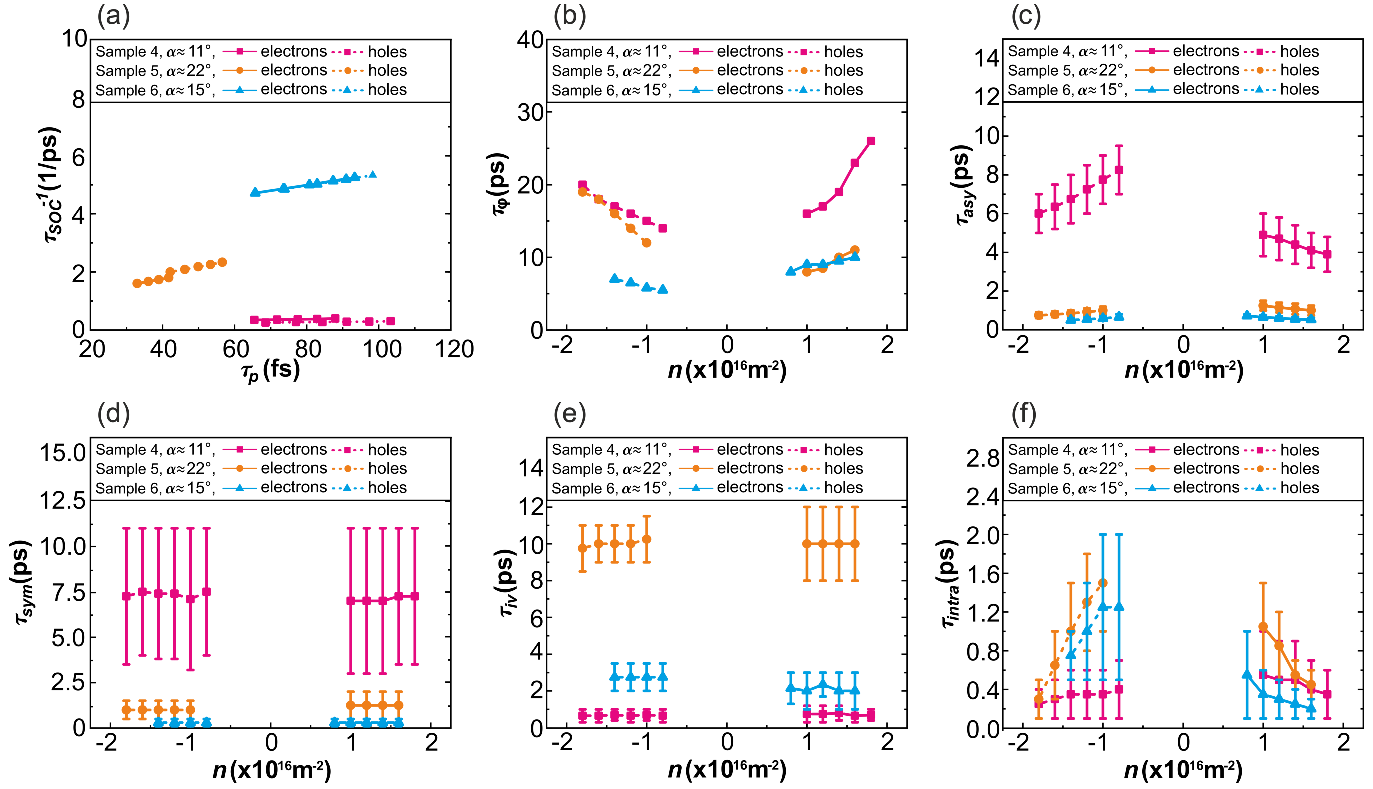


FIG. S 4. (a) $\tau_{SOC}^{-1}$ as a function of the momentum relaxation time $\tau_p$ for samples 4-6 in the electron and hole regimes. The linear progression of the curves and the similar slope of the curves for both regimes are particularly striking. For the calculation of $\tau_{SOC}^{-1}$ the average values of $\tau_{asy}$ and $\tau_{sym}$ were used. (b) the progression of the phase coherence time $\tau_\phi$ as a function of the charge carrier density $n$. $\tau_\phi$ always increases with increasing $n$. (c) and (d) the progression of $\tau_{asy}$ and $\tau_{sym}$ for samples 4-6 for different $n$. $\tau_{asy}$ shows a dependence on $n$, whereas $\tau_{sym}$ does not. First signs of an angular dependence can also be seen for both parameters. (e)-(f) intervalley scattering time $\tau_{iv}$ and intravalley scattering time $\tau_{intra}$ for samples 4-6 as a function of $n$. Here $\tau_{iv}$ shows no dependence on $n$. $\tau_{intra}$ on the other hand decreases with increasing $n$. An angle dependence is not recognizable here.

## S.2.
## FURTHER DATA - PRESSURE CELL STUDIES

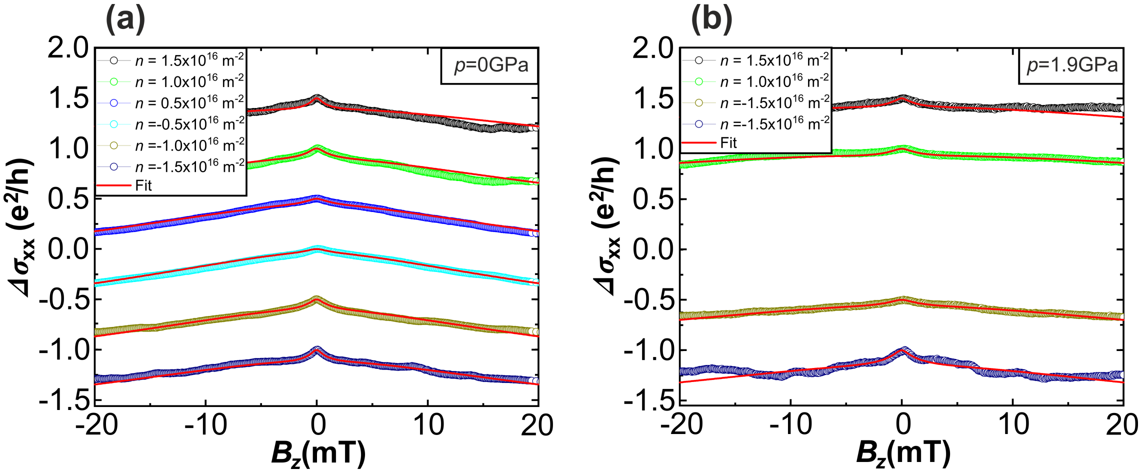


FIG. S 5. (a)-(b) measurements of the quantum mechanical correction of the conductivity $\Delta\sigma_{xx}$ as a function of the external magnetic field $B_z$ for the two cases ($p = 0\,\text{GPa}$ and $p = 2\,\text{GPa}$). The red curves are the corresponding fits. In b), the curves for the charge carrier densities $n = \pm 0.5 \times 10^{16}\,\text{m}^{-2}$ are missing, as no transport parameters were available for them.
